# Supplementary material for: TRIER: Template-Guided Neural Networks for Robust and Interpretable Sleep Stage Identification from EEG Recordings
Source: arXiv:2009.05407 source file (2020-09-10)
Supplement: Supplementary file 1 [file 00_Appendix.tex]

\section{Dataset Statistics}
\subsection{Class Ratio}

\begin{table}[]
  \caption{Class Distributions for each Datasets}
  \centering
  \begin{tabular}{@{} l@{\hskip 0.3in}c@{\hskip 0.15in}c@{\hskip 0.15in}c@{\hskip 0.15in}c@{\hskip 0.15in}c @{}}
    \toprule
    Datasets                       & W            & N1         & N2         & N3        & REM    \\
    \midrule[0.7pt]
    EDF-2013                       & 8285         & 2804       & 17799      & 5703      & 7717   \\
    EDF-2018                       & 65795        & 21469      & 68633      & 12991     & 25767  \\
    ISRUC Group1                   & 20098        & 11062      & 27511      & 17251     & 11265  \\
    ISRUC Group3                   & 1674         & 1217       & 2616       & 2016      & 1066   \\
    CAP                            & 18828        & 4439       & 36937      & 24092     & 17672  \\
    SVUH-UCD                       & 2140         & 1604       & 3173       & 1225      & 1411   \\
    \bottomrule
  \end{tabular}
  \label{tab:supp_class_ratio}
\end{table}

\subsection{Scale Information}

\section{Classification Performances}
\subsection{Quantile-scaled Sleep-EDF Classification}

\begin{table}[]
  \caption{Sleep-EDF Dataset}
  \label{tab:supp_edf2018}
  \centering
  \begin{tabular}{@{}cl@{\hskip 0.05in}ccc@{\hskip 0.015in}cc@{}}
    \toprule
    &                   & \multicolumn{2}{c}{EDF-2013}                               & 
                        & \multicolumn{2}{c}{EDF-2018}                           \\
                        \cmidrule(lr){3-4} \cmidrule(lr){6-7}
    & Methods           & Macro-F1                       & Accuracy                      &
                        & Macro-F1                       & Accuracy                      \\
    \midrule[0.7pt]
    \multirow{2}{*}{LSTM}
    & \textbf{Template} & 0.77461                        & 0.82384                       &
                        & 0.72822                        & 0.76571                       \\
    & Baseline          & 0.75793                        & 0.80293                       &
                        & 0.71408                        & 0.75728                       \\
    \bottomrule
  \end{tabular}
\end{table}

\subsection{Class-wise F1 scores}
\begin{table}[]
  \caption{EDF 2018 Dataset}
  \centering
  \begin{tabular}{@{} cl ccccc @{}}
    \toprule
    &                               & \multicolumn{5}{c}{Class F1-Score} \\
    \cmidrule(l){3-7} 
    & Methods                       & W            & N1         & N2         & N3        & REM    \\
    \midrule[0.7pt]
    \multirow{2}{*}{LSTM}
    & \textbf{Template}             & 0.8638       & 0.4473     & 0.8057     & 0.7636    & 0.7557 \\
    & Baseline                      & 0.8620       & 0.4396     & 0.7867     & 0.7536    & 0.7689 \\
    \bottomrule
  \end{tabular}
  \label{tab:supp_f1_edf2018}
\end{table}

\begin{table}[]
  \caption{ISRUC Group 1 Dataset}
  \centering
  \begin{tabular}{@{} cl ccccc @{}}
    \toprule
    &                               & \multicolumn{5}{c}{Class F1-Score} \\
    \cmidrule(l){3-7} 
    & Methods                       & W            & N1         & N2         & N3        & REM  \\
    \midrule[0.7pt]
    \multirow{2}{*}{LSTM}
    & Template                      & 0.8456       & 0.5177     & 0.7585     & 0.8529    & 0.7717 \\
    & Baseline                      & 0.8204       & 0.5098     & 0.7238     & 0.8575    & 0.7517 \\
    \bottomrule
  \end{tabular}
  \label{tab:supp_f1_isruc}
\end{table}

\begin{table}[]
  \caption{CAP Dataset}
  \centering
  \begin{tabular}{@{} cl ccccc @{}}
    \toprule
    &                               & \multicolumn{5}{c}{Class F1-Score} \\
    \cmidrule(l){3-7} 
    & Methods                       & W            & N1         & N2         & N3        & REM    \\
    \midrule[0.7pt]
    \multirow{2}{*}{LSTM}
    & \textbf{Template}             & 0.8314       & 0.4091     & 0.7889     & 0.8267    & 0.7923 \\
    & Baseline                      & 0.8037       & 0.3733     & 0.7406     & 0.8083    & 0.7815 \\
    \bottomrule
  \end{tabular}
  \label{tab:supp_f1_cap}
\end{table}

\subsection{Per-class Analysis: Confusion Matrix}
